# Supplementary material for: DualApp: Tight Over-Approximation for Neural Network Robustness Verification via Under-Approximation
Source: arXiv:2211.11186 source file (2022-11-21)
Supplement: Supplementary file 1 [file appendix.tex]

\section{Additional Experimental Results}

% This section presents the additional experimental results, including the comparison of Sampling-version DualApp with NeWise,  DeepCert, VeriNet and RobustVerifier on 17 Tanh, 18 Arctan, and 16 Sigmoid models trained on Mnist, Fashion Mnist and Cifar with different structures.

\begin{table*}[h!]
\centering
\caption{Additional Comparison result I: Comparison results of sampling-version DualApp (D.U.$_{sp}$) and existing tools, NeWise (N.W.), DeepCert (D.C.), VeriNet (V.N.) and RobustVerifier (R.V.) on 17 Tanh networks.}
\setlength{\tabcolsep}{4.5pt}
\begin{tabular}{|l|r|r|r|r|r|r|r|r|r|r|r|r|r|}
\hline
\multirow{2}{*}{Database}                                                 & \multirow{2}{*}{Model}                                       & \multirow{2}{*}{Nodes} & D.U.$_{sp}$ & N.W.  & \multirow{2}{*}{\begin{tabular}[c]{@{}l@{}}Impro.\\ (\%)\end{tabular}} & D.C. & \multirow{2}{*}{\begin{tabular}[c]{@{}l@{}}Impro.\\ (\%)\end{tabular}} & V.N. & \multirow{2}{*}{\begin{tabular}[c]{@{}l@{}}Impro.\\ (\%)\end{tabular}} & \begin{tabular}[c]{@{}l@{}}R.V.\end{tabular} & \multirow{2}{*}{\begin{tabular}[c]{@{}l@{}}Impro.\\ (\%)\end{tabular}} & \multirow{2}{*}{\begin{tabular}[c]{@{}l@{}}D.U.$_{sp}$ \\ Time (s)\end{tabular}} & \multirow{2}{*}{Others Time(s)}   \\ \cline{4-5} \cline{7-7} \cline{9-9} \cline{11-11}
                                                                          &                                                              &                        & Bounds   & Bounds  &                                                                        & Bounds   &                                                                        & Bounds  &                                                                        & Bounds                                                    &                                                                        &                                                                               &                                   \\ \hline
\multirow{6}{*}{Mnist}                     \setlength{\tabcolsep}{2pt}                               & \begin{tabular}[c]{@{}l@{}}${\rm CNN}_{3-2}$\end{tabular} & 2,514                  & 0.02677  & 0.02558 & 4.65                                                                   & 0.02618  & 2.25                                                                   & 0.02622 & 2.10                                                                   & 0.02565                                                   & 4.37                                                                   & 3.34                                                                          & 0.16   \textpm 0.02    \\ 
                                                                          &   ${\rm FNN}_{3\times 50}$                                                        & 160                    & 0.00545  & 0.00456 & 19.52                                                                  & 0.00529  & 3.02                                                                   & 0.00536 & 1.68                                                                   & 0.00439                                                   & 24.15                                                                  & 3.02                                                                          & 0.14   \textpm 0.00    \\ 
                                                                          & ${\rm FNN}_{3\times 100}$                                                       & 310                    & 0.00623  & 0.00499 & 24.85                                                                  & 0.00609  & 2.30                                                                   & 0.00616 & 1.14                                                                   & 0.00512                                                   & 21.68                                                                  & 5.28                                                                          & 0.37   \textpm 0.01    \\ 
                                                                          & ${\rm FNN}_{3\times 200}$                                                        & 610                    & 0.00676  & 0.00508 & 33.07                                                                  & 0.00663  & 1.96                                                                   & 0.00669 & 1.05                                                                   & 0.00557                                                   & 21.36                                                                  & 10.42                                                                          & 1.19   \textpm 0.05    \\ 
                                                                          & ${\rm FNN}_{3\times 400}$                                                        & 1,210                  & 0.00672  & 0.00479 & 40.29                                                                  & 0.00660   & 1.82                                                                   & 0.00667 & 0.75                                                                   & 0.00553                                                   & 21.52                                                                  & 24.28                                                                         & 4.63   \textpm 0.12    \\ 
                                                                          & ${\rm FNN}_{3\times 700}$                                                        & 2,110                  & 0.00665  & 0.00459 & 44.88                                                                  & 0.00650   & 2.31                                                                   & 0.00660  & 0.76                                                                   & 0.00537                                                   & 23.84                                                                  & 50.48                                                                         & 12.27   \textpm 0.43   \\  \hline
\multirow{7}{*}{\begin{tabular}[c]{@{}l@{}}Fashion \\ Mnist\end{tabular}} & \begin{tabular}[c]{@{}l@{}}${\rm CNN}_{3-2}$\end{tabular} & 2514   & 0.09247 & 0.09091 & 1.72  & 0.08805 & 5.02 & 0.08772 & 5.41 & 0.08387 & 10.25                                                                   & 3.22                                                                          & 0.15   \textpm 0.02    \\ 
                                                                          & \begin{tabular}[c]{@{}l@{}}${\rm CNN}_{3-4}$\end{tabular} & 5018   & 0.07704 & 0.07452 & 3.38  & 0.0729  & 5.68 & 0.07295 & 5.61 & 0.06848 & 12.50                                                                   & 5.68                                                                          & 0.26   \textpm 0.05    \\  
                                                                          & ${\rm FNN}_{3\times 50}$                                                         & 160    & 0.01035 & 0.00915 & 13.11 & 0.01013 & 2.17 & 0.0102  & 1.47 & 0.00858 & 20.63                                                                  & 3.87                                                                          & 0.20   \textpm 0.01    \\ 
                                                                          & ${\rm FNN}_{3\times 100}$                                                        & 310    & 0.00921 & 0.00797 & 15.56 & 0.00907 & 1.54 & 0.00911 & 1.10 & 0.00778 & 18.38                                                                  & 6.33                                                                          & 0.57   \textpm 0.12    \\  
                                                                          & ${\rm FNN}_{3\times 700}$                                                        & 2,110  & 0.00757 & 0.00634 & 19.40 & 0.00749 & 1.07 & 0.00751 & 0.80 & 0.00666 & 13.66                                                                  & 78.02                                                                         & 13.44   \textpm 0.62   \\  \hline
\multirow{4}{*}{Cifar-10}                                                 & \begin{tabular}[c]{@{}l@{}}${\rm CNN}_{3-4}$\end{tabular} & 5018   & 0.02551 & 0.02469 & 3.32  & 0.02528 & 0.91 & 0.02523 & 1.11 & 0.02492 & 2.37                                                                   & 6.02                                                                          & 0.26   \textpm 0.05    \\ 
                                                                           
                                                                          & ${\rm CNN}_{4-5}$          & 8690   & 0.01942 & 0.01863 & 4.24  & 0.01917 & 1.30 & 0.01912 & 1.57 & 0.01887 & 2.91                                                                  & 7.79                                                                          & 1.73   \textpm 0.24    \\  
                                                                           
                                                                          & ${\rm FNN}_{3\times 50}$                                                         & 160                    & 0.00287  & 0.00232 & 23.71                                                                  & 0.00285  & 0.70                                                                   & 0.00285 & 0.70                                                                   & 0.00254                                                   & 12.99                                                                  & 7.79                                                                          & 1.73   \textpm 0.24    \\ 
                                                                          & ${\rm FNN}_{3\times 100}$                                                        & 310                    & 0.00253  & 0.00194 & 30.41                                                                  & 0.00251  & 0.80                                                                   & 0.00251 & 0.80                                                                   & 0.00225                                                   & 12.44                                                                  & 19.47                                                                          & 10.45   \textpm 4.36   \\ 
                                                                          & ${\rm FNN}_{3\times 700}$                                                        & 2,110                  & 0.00229  & 0.00155 & 47.74                                                                  & 0.00226  & 1.33                                                                   & 0.00228 & 0.44                                                                   & 0.00201                                                   & 13.93                                                                  & 122.89                                                                         & 66.01   \textpm 12.74 \\  \hline
\end{tabular}
\end{table*}
\vspace{-2mm}

\begin{table*}[h!]
\centering
\caption{Additional Comparison results II: Comparison of sampling-version DualApp (D.U.$_{sp}$) and existing tools, NeWise (N.W.), DeepCert (D.C.), VeriNet (V.N.) and RobustVerifier (R.V.) on 18 Arctan networks.}
\setlength{\tabcolsep}{4.5pt}
\begin{tabular}{|l|r|r|r|r|r|r|r|r|r|r|r|r|r|}
\hline
\multirow{2}{*}{Database}                                                  & \multirow{2}{*}{Model}                                       & \multirow{2}{*}{Nodes} & D.U.$_{sp}$ & N.W.  & \multirow{2}{*}{\begin{tabular}[c]{@{}l@{}}Impro.\\ (\%)\end{tabular}} & D.C. & \multirow{2}{*}{\begin{tabular}[c]{@{}l@{}}Impro.\\ (\%)\end{tabular}} & V.N. & \multirow{2}{*}{\begin{tabular}[c]{@{}l@{}}Impro.\\ (\%)\end{tabular}} & \begin{tabular}[c]{@{}l@{}}R.V.\end{tabular} & \multirow{2}{*}{\begin{tabular}[c]{@{}l@{}}Impro.\\ (\%)\end{tabular}} & \multirow{2}{*}{\begin{tabular}[c]{@{}l@{}}D.U.$_{sp}$\end{tabular}} & \multirow{2}{*}{Others Time(s)}   \\ \cline{4-5} \cline{7-7} \cline{9-9} \cline{11-11}
                                                                           &                                                              &                        & Bounds   & Bounds  &                                                                        & Bounds   &                                                                        & Bounds  &                                                                        & Bounds                                                    &                                                                        &                                                                               &                                   \\ \hline
\multirow{6}{*}{Mnist}                                                     & \begin{tabular}[c]{@{}l@{}}${\rm CNN}_{3-2}$\end{tabular}  & 2,514                  & 0.01920   & 0.01821 & 5.44                                                                   & 0.01836  & 4.58                                                                   & 0.01896 & 1.27                                                                   & 0.01829                                                   & 4.98                                                                   & 2.78                                                                          & 0.15   \textpm 0.02    \\  
                                                                           & ${\rm FNN}_{3\times 50}$                                                         & 160                    & 0.00568  & 0.00481 & 18.09                                                                  & 0.00437  & 29.98                                                                  & 0.00558 & 1.79                                                                   & 0.00465                                                   & 22.15                                                                  & 3.02                                                                          & 0.16   \textpm 0.02    \\ 
                                                                           & ${\rm FNN}_{3\times 100}$                                                        & 310                    & 0.00635  & 0.00518 & 22.59                                                                  & 0.00495  & 28.28                                                                  & 0.00627 & 1.28                                                                   & 0.00529                                                   & 20.04                                                                  & 5.11                                                                          & 0.37   \textpm 0.04    \\ 
                                                                           & ${\rm FNN}_{3\times 200}$                                                        & 610                    & 0.00716  & 0.00547 & 30.90                                                                  & 0.00554  & 29.24                                                                  & 0.00708 & 1.13                                                                   & 0.00587                                                   & 21.98                                                                  & 10.34                                                                          & 1.20   \textpm 0.02    \\ 
                                                                           & ${\rm FNN}_{3\times 400}$                                                        & 1,210                  & 0.00733  & 0.00528 & 38.83                                                                  & 0.00551  & 33.03                                                                  & 0.00725 & 1.10                                                                   & 0.00589                                                   & 24.45                                                                  & 25.46                                                                         & 4.65   \textpm 0.42    \\ 
                                                                           & ${\rm FNN}_{3\times 700}$                                                        & 2,110                  & 0.00721  & 0.00506 & 42.49                                                                  & 0.00532  & 35.53                                                                  & 0.00713 & 1.12                                                                   & 0.00572                                                   & 26.05                                                                  & 50.98                                                                         & 12.18   \textpm 0.23   \\  \hline
\multirow{7}{*}{\begin{tabular}[c]{@{}l@{}}Fashion \\ Mnist\end{tabular}} & \begin{tabular}[c]{@{}l@{}}${\rm CNN}_{3-2}$\end{tabular}  & 2,514                  & 0.03006  & 0.02839 & 5.88                                                                   & 0.02584  & 16.33                                                                  & 0.02930  & 2.59                                                                   & 0.02811                                                   & 6.94                                                                   & 2.86                                                                          & 0.15   \textpm 0.01    \\ 
                                                                           & \begin{tabular}[c]{@{}l@{}}${\rm CNN}_{3-4}$\end{tabular} & 5,018                  & 0.03430   & 0.03125 & 9.76                                                                   & 0.03084  & 11.22                                                                  & 0.03390  & 1.18                                                                   & 0.03094                                                   & 10.86                                                                  & 5.92                                                                          & 0.28   \textpm 0.03    \\  
                                                                           & ${\rm FNN}_{3\times 50}$                                                         & 160                    & 0.00574  & 0.00476 & 20.59                                                                  & 0.00447  & 28.41                                                                  & 0.00565 & 1.59                                                                   & 0.00476                                                   & 20.59                                                                  & 3.15                                                                         & 0.14   \textpm 0.01    \\ 
                                                                           & ${\rm FNN}_{3\times 100}$                                                        & 310                    & 0.00497  & 0.00391 & 27.11                                                                  & 0.00387  & 28.42                                                                  & 0.00490  & 1.43                                                                   & 0.00471                                                   & 5.52                                                                   & 5.32                                                                          & 0.42   \textpm 0.08    \\ 
                                                                           & ${\rm FNN}_{3\times 200}$                                                        & 610                    & 0.00471  & 0.00349 & 34.96                                                                  & 0.00358  & 31.56                                                                  & 0.00466 & 1.07                                                                   & 0.00390                                                    & 20.77                                                                  & 10.56                                                                          & 1.20   \textpm 0.06    \\ 
                                                                           & ${\rm FNN}_{3\times 400}$                                                        & 1210                   & 0.00442  & 0.00312 & 41.67                                                                  & 0.00322  & 37.27                                                                  & 0.00437 & 1.14                                                                   & 0.00355                                                   & 24.51                                                                  & 25.22                                                                         & 4.20   \textpm 0.21    \\ 
                                                                           & ${\rm FNN}_{3\times 700}$                                                        & 2,110                  & 0.00408  & 0.00284 & 43.66                                                                  & 0.00290   & 40.69                                                                  & 0.00401 & 1.75                                                                   & 0.00318                                                   & 28.30                                                                  & 50.12                                                                         & 12.14   \textpm 0.39   \\  \hline
\multirow{5}{*}{Cifar-10}                                                  & \begin{tabular}[c]{@{}l@{}}${\rm CNN}_{3-4}$\end{tabular}  & 5,018                  & 0.01136  & 0.01064 & 6.77                                                                   & 0.01067  & 6.47                                                                   & 0.01133 & 0.26                                                                   & 0.01118                                                   & 1.61                                                                   & 4.87                                                                          & 0.28   \textpm 0.03    \\  
                                                                           & ${\rm FNN}_{3\times 50}$                                                         & 160                    & 0.00323  & 0.00262 & 23.28                                                                  & 0.00266  & 21.43                                                                  & 0.00321 & 0.62                                                                   & 0.00283                                                   & 14.13                                                                  & 7.26                                                                          & 1.67   \textpm 0.16    \\ 
                                                                           & ${\rm FNN}_{3\times 100}$                                                        & 310                    & 0.00277  & 0.00216 & 28.24                                                                  & 0.00220   & 25.91                                                                  & 0.00275 & 0.73                                                                   & 0.00248                                                   & 11.69                                                                  & 13.88                                                                         & 4.33\textpm   0.88     \\ 
                                                                           & ${\rm FNN}_{3\times 200}$                                                       & 610                    & 0.00255  & 0.00189 & 34.92                                                                  & 0.00196  & 30.10                                                                  & 0.00253 & 0.79                                                                   & 0.00228                                                   & 11.84                                                                  & 27.94                                                                         & 10.48   \textpm 1.56   \\ 
                                                                           & ${\rm FNN}_{3\times 700}$                                                        & 2,110                  & 0.00246  & 0.00167 & 47.31                                                                  & 0.00179  & 37.43                                                                  & 0.00245 & 0.41                                                                   & 0.00212                                                   & 16.04                                                                  & 79.10                                                                         & 36.44   \textpm 3.85   \\  \hline
\end{tabular}
\end{table*}
\vspace{-2mm}

\begin{table*}[h!]
\centering
\caption{Additional Comparison result III: Comparison of sampling-version DualApp (D.U.$_{sp}$) and existing tools, NeWise (N.W.), DeepCert (D.C.), VeriNet (V.N.) and RobustVerifier (R.V.) on 16 Sigmoid networks.}
\setlength{\tabcolsep}{4.5pt}
\begin{tabular}{|l|r|r|r|r|r|r|r|r|r|r|r|r|r|}
\hline
\multirow{2}{*}{Database}                                                  & \multirow{2}{*}{Model}                                       & \multirow{2}{*}{Nodes} & D.U.$_{sp}$ & N.W.  & \multirow{2}{*}{\begin{tabular}[c]{@{}l@{}}Impro.\\ (\%)\end{tabular}} & D.C. & \multirow{2}{*}{\begin{tabular}[c]{@{}l@{}}Impro.\\ (\%)\end{tabular}} & V.N. & \multirow{2}{*}{\begin{tabular}[c]{@{}l@{}}Impro.\\ (\%)\end{tabular}} & \begin{tabular}[c]{@{}l@{}}R.V.\end{tabular} & \multirow{2}{*}{\begin{tabular}[c]{@{}l@{}}Impro.\\ (\%)\end{tabular}} & \multirow{2}{*}{\begin{tabular}[c]{@{}l@{}}D.U.$_{sp}$ \\ Time (s)\end{tabular}} & \multirow{2}{*}{Others Time(s)}   \\ \cline{4-5} \cline{7-7} \cline{9-9} \cline{11-11}
                                                                           &                                                              &                        & Bounds   & Bounds  &                                                                        & Bounds   &                                                                        & Bounds  &                                                                        & Bounds                                                    &                                                                        &                                                                               &                                   \\ \hline
\multirow{5}{*}{Mnist}                                                     & \begin{tabular}[c]{@{}l@{}}${\rm CNN}_{3-2}$\end{tabular}  & 2,514                  & 0.06119   & 0.06074 & 0.74                                                                & 0.05789 & 5.70                                                                  &  0.05803    & 5.45                                                                   & 0.05686                                                   & 7.62                                                                   & 2.81                                                                          & 0.15   \textpm 0.02    \\  
                                                                           & ${\rm CNN}_{3-4}$          & 5018   & 0.04875 & 0.04776 & 2.07  & 0.04721 & 3.26 & 0.04715 & 3.39 & 0.04639 & 5.09                                                                  & 3.44                                                                          & 0.15   \textpm 0.02    \\ 
                                                                           & ${\rm CNN}_{4-5}$          & 8690   & 0.04863 & 0.04763 & 2.10  & 0.04551 & 6.86 & 0.04548 & 6.93 & 0.04355 & 11.66                                                                  & 15.33                                                                          & 0.89   \textpm 0.03    \\ 
                                                                           & ${\rm FNN}_{3 \times 50}$  & 160    & 0.00779 & 0.00693 & 12.41 & 0.0076  & 2.50 & 0.00768 & 1.43 & 0.00649 & 20.03                                                                  & 3.28                                                                          & 0.15   \textpm 0.02    \\ 
                                                                           & ${\rm FNN}_{3 \times 100}$ & 310    & 0.00885 & 0.00777 & 13.90 & 0.00858 & 3.15 & 0.00871 & 1.61 & 0.00744 & 18.95                                                                  & 5.46                                                                         & 0.22   \textpm 0.02    \\   \hline
\multirow{7}{*}{\begin{tabular}[c]{@{}l@{}}Fashion \\ Mnist\end{tabular}} & \begin{tabular}[c]{@{}l@{}}${\rm CNN}_{3-2}$\end{tabular}  & 2,514                  & 0.03006  & 0.02839 & 5.88                                                                   & 0.02584  & 16.33                                                                  & 0.02930  & 2.59                                                                   & 0.02811                                                   & 6.94                                                                   & 2.86                                                                          & 0.15   \textpm 0.01    \\ 
                                                                           & \begin{tabular}[c]{@{}l@{}}${\rm CNN}_{3-4}$\end{tabular} & 5,018                  & 0.03430   & 0.03125 & 9.76                                                                   & 0.03084  & 11.22                                                                  & 0.03390  & 1.18                                                                   & 0.03094                                                   & 10.86                                                                  & 5.92                                                                          & 0.28   \textpm 0.03    \\  
                                                                           & ${\rm FNN}_{3\times 50}$                                                         & 160                    & 0.00574  & 0.00476 & 20.59                                                                  & 0.00447  & 28.41                                                                  & 0.00565 & 1.59                                                                   & 0.00476                                                   & 20.59                                                                  & 3.15                                                                         & 0.14   \textpm 0.01    \\ 
                                                                           & ${\rm FNN}_{3\times 100}$                                                        & 310                    & 0.00497  & 0.00391 & 27.11                                                                  & 0.00387  & 28.42                                                                  & 0.00490  & 1.43                                                                   & 0.00471                                                   & 5.52                                                                   & 5.32                                                                          & 0.42   \textpm 0.08    \\  
                                                                           & ${\rm FNN}_{3\times 400}$                                                        & 1210                   & 0.00442  & 0.00312 & 41.67                                                                  & 0.00322  & 37.27                                                                  & 0.00437 & 1.14                                                                   & 0.00355                                                   & 24.51                                                                  & 25.22                                                                         & 4.20   \textpm 0.21    \\ 
                                                                           & ${\rm FNN}_{3\times 700}$                                                        & 2,110                  & 0.00408  & 0.00284 & 43.66                                                                  & 0.00290   & 40.69                                                                  & 0.00401 & 1.75                                                                   & 0.00318                                                   & 28.30                                                                  & 50.12                                                                         & 12.14   \textpm 0.39   \\  \hline
\multirow{5}{*}{Cifar-10}                                                  & \begin{tabular}[c]{@{}l@{}}${\rm CNN}_{3-4}$\end{tabular}  & 5,018                  & 0.01136  & 0.01064 & 6.77                                                                   & 0.01067  & 6.47                                                                   & 0.01133 & 0.26                                                                   & 0.01118                                                   & 1.61                                                                   & 4.87                                                                          & 0.28   \textpm 0.03    \\  
                                                                           & ${\rm CNN}_{4-5}$          & 8690   & 0.01942 & 0.01863 & 4.24  & 0.01917 & 1.30 & 0.01912 & 1.57 & 0.01887 & 2.91                                                                  & 17.22                                                                          & 1.17   \textpm 0.08    \\ 
                                                                           & ${\rm FNN}_{3\times 50}$                                                         & 160    & 0.00455 & 0.00406 & 12.07 & 0.00454 & 0.22 & 0.00452 & 0.66 & 0.00415 & 9.64                                                                  & 6.68                                                                          & 2.07   \textpm 0.26    \\ 
                                                                           & ${\rm FNN}_{3\times 100}$                                                        & 310    & 0.00469 & 0.00401 & 16.96 & 0.00468 & 0.21 & 0.00466 & 0.64 & 0.00426 & 10.09                                                                  & 12.23                                                                         & 3.98\textpm   0.84     \\ 
                                                                           & ${\rm FNN}_{3\times 200}$                                                       & 610    & 0.00408 & 0.00344 & 18.60 & 0.00407 & 0.25 & 0.00406 & 0.49 & 0.00377 & 8.22                                                                  & 30.27                                                                         & 12.82   \textpm 2.11   \\   \hline
\end{tabular}
\end{table*}

\begin{figure*}
	\centering
	\begin{subfigure}{0.32\textwidth}
		\includegraphics[width=\textwidth]{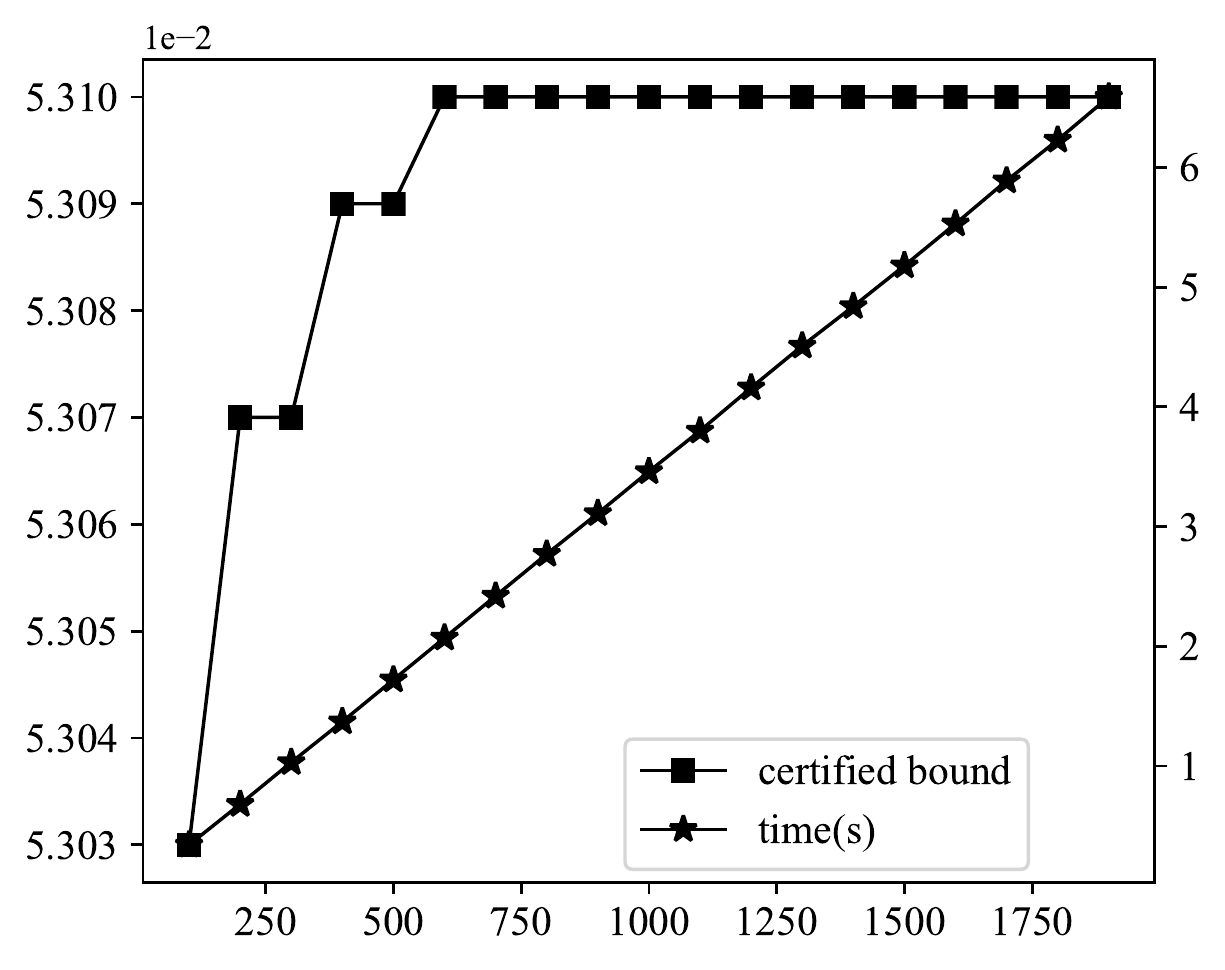}
		\caption{Sampling-based results on $\rm{CNN}_{2-3}$ trained on Mnist.}
		\label{fig:Sampling_mnist_cnn}
	\end{subfigure}
	\hfill
	\begin{subfigure}{0.32\textwidth}
		\includegraphics[width=\textwidth]{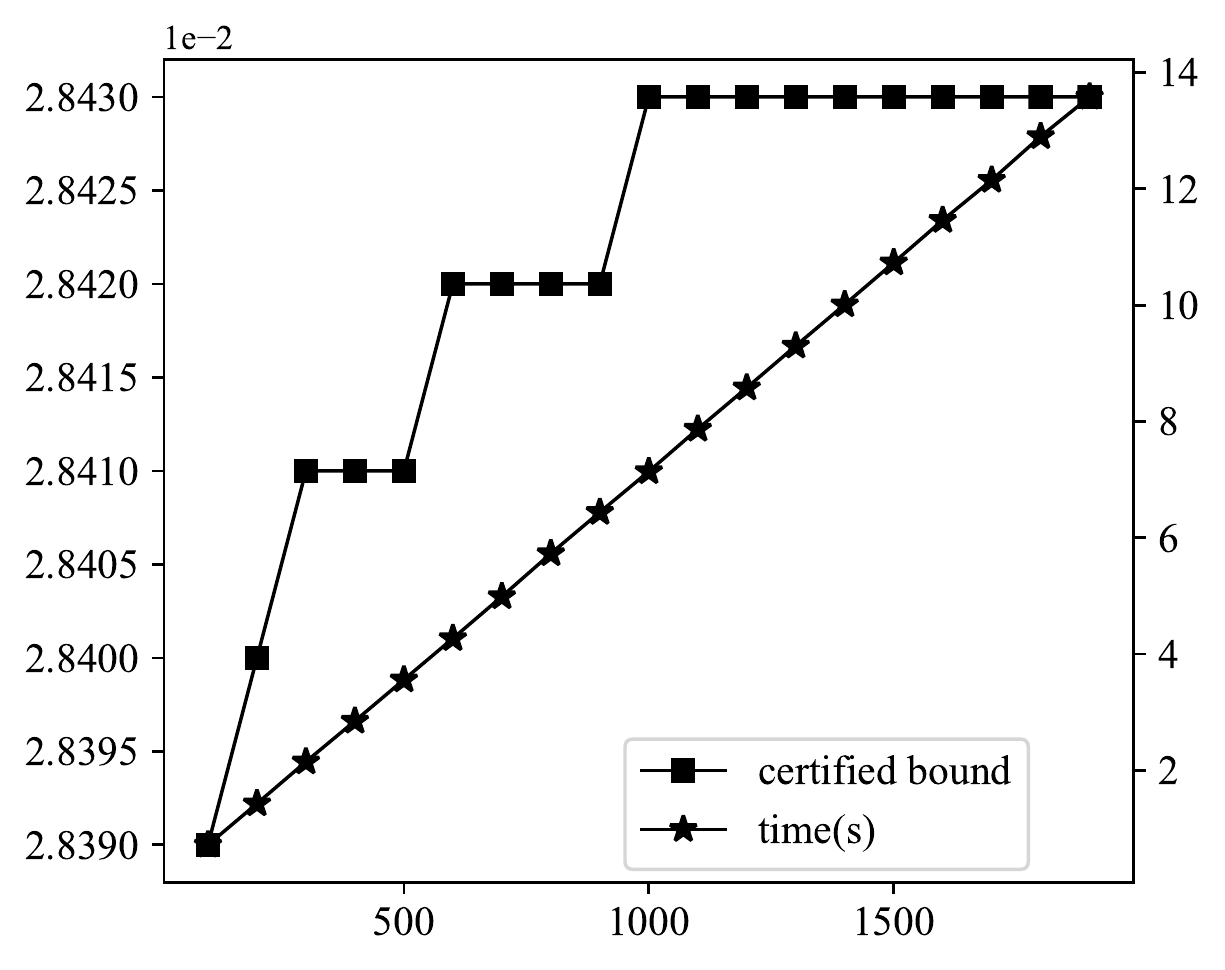}
		\caption{Sampling-based results on $\rm{FNN}_{1\times 200}$ trained on Mnist.}
		\label{fig:Sampling_mnist_fnn}
	\end{subfigure}
	\hfill
	\begin{subfigure}{0.32\textwidth}
		\includegraphics[width=\textwidth]{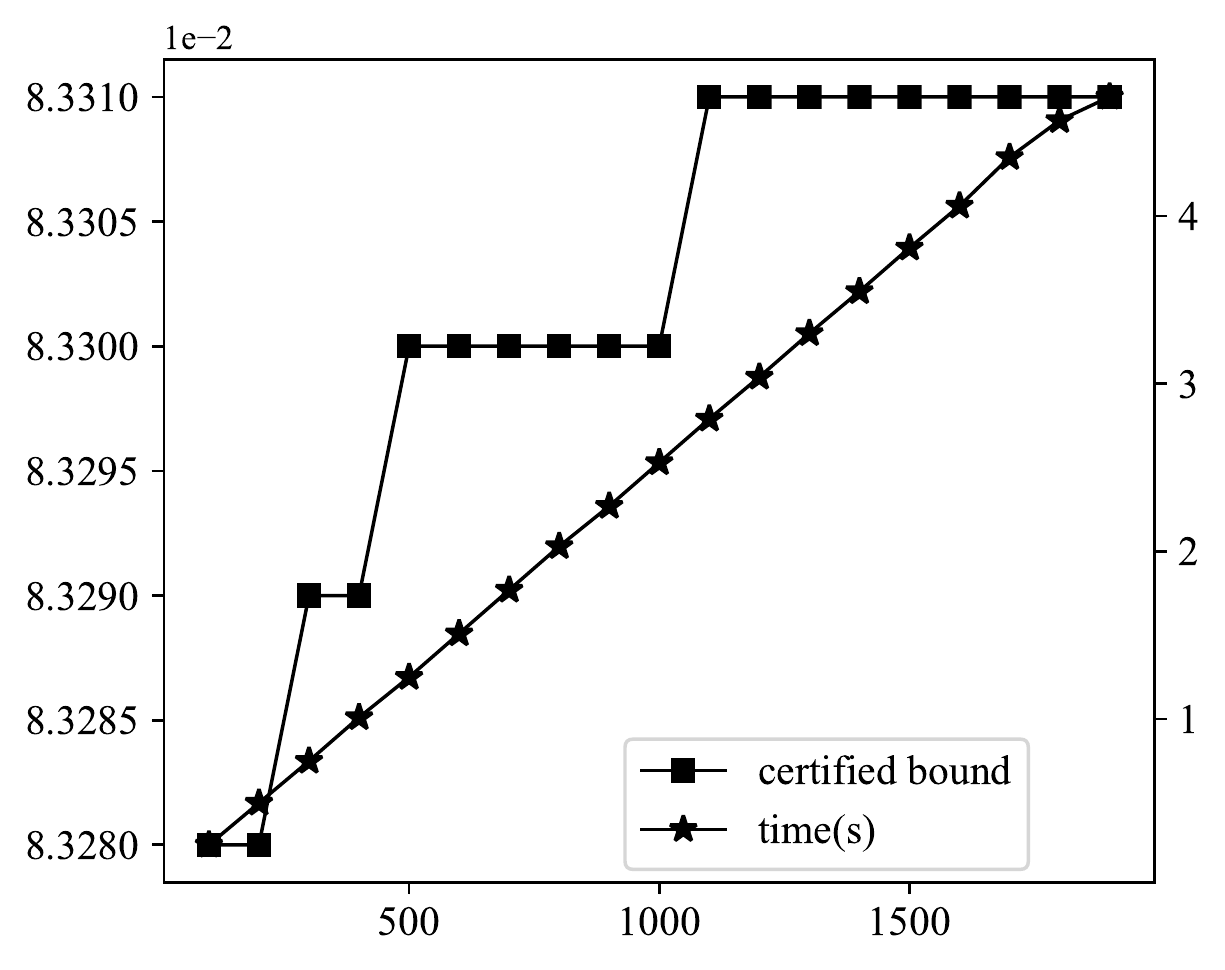}
		\caption{Sampling-based results on $\rm{CNN}_{2-2}$  trained on Fashion Mnist.}
		\label{fig:Sampling_fashion_mnist_cnn}
	\end{subfigure}
	\hfill\\
% 	\begin{subfigure}{0.24\textwidth}
% 		\includegraphics[width=\textwidth]{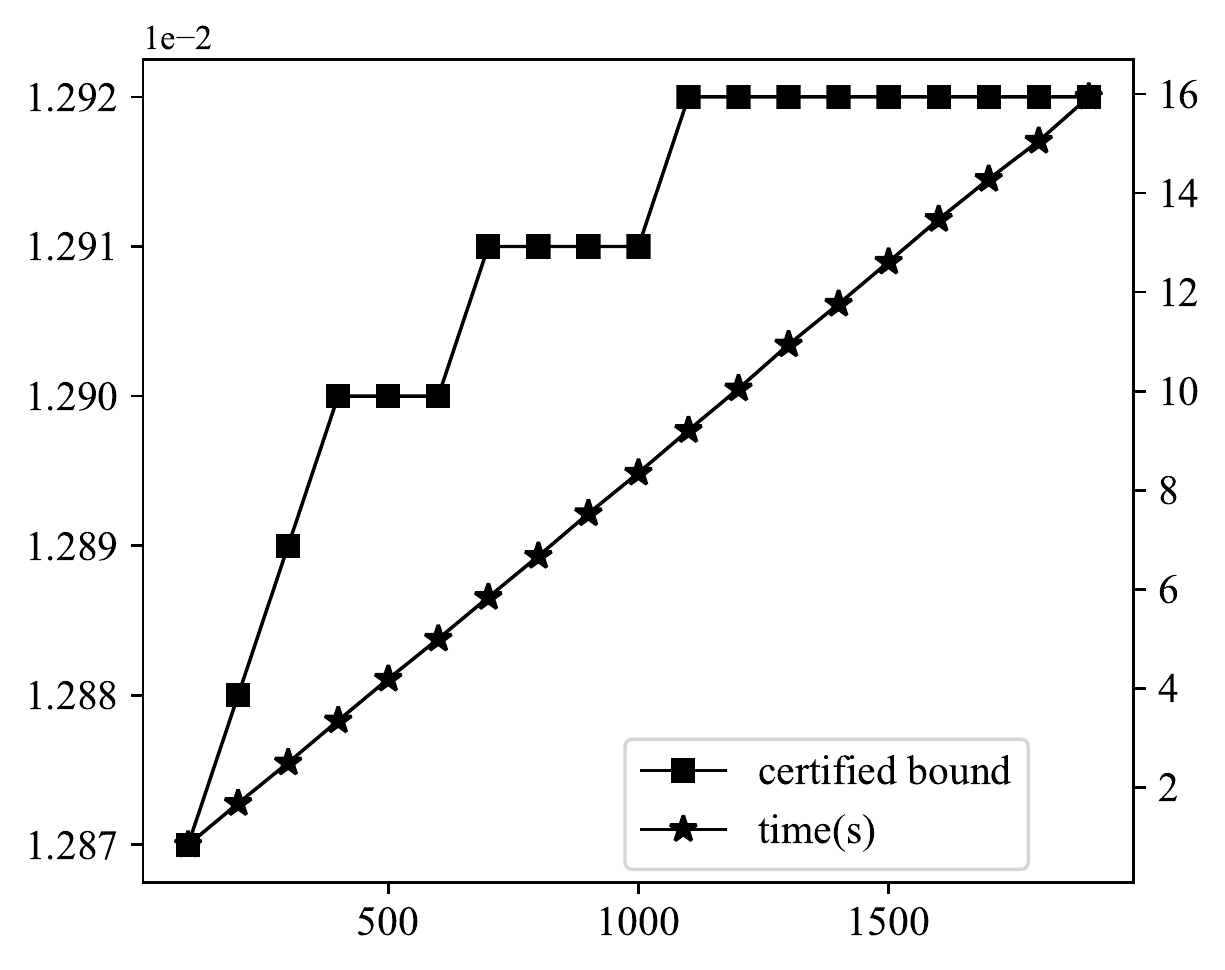}
% 		\caption{Sampling-based results on $\rm{FNN}_{1\times 100}$  trained on Fashion Mnist.}
% 		\label{fig:Sampling_fashion_mnist_fnn}
% 	\end{subfigure}
% 	\hfill
    
	\begin{subfigure}{0.32\textwidth}
		\includegraphics[width=\textwidth]{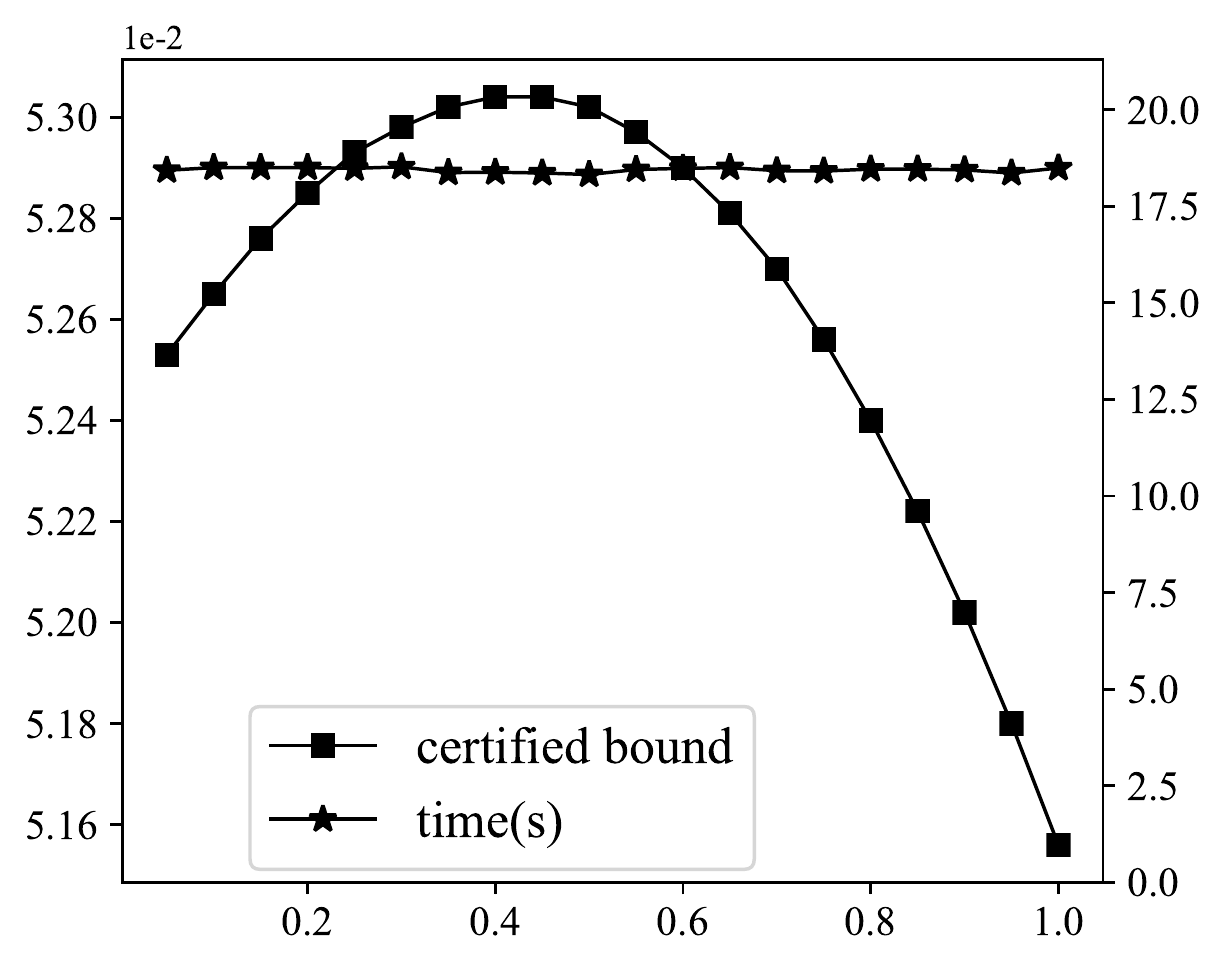}
		\caption{Gradient-based results on $\rm{CNN}_{2-3}$ trained on Mnist.}
		\label{fig:GD_mnist_cnn}
	\end{subfigure}
	\hfill
	\begin{subfigure}{0.32\textwidth}
		\includegraphics[width=\textwidth]{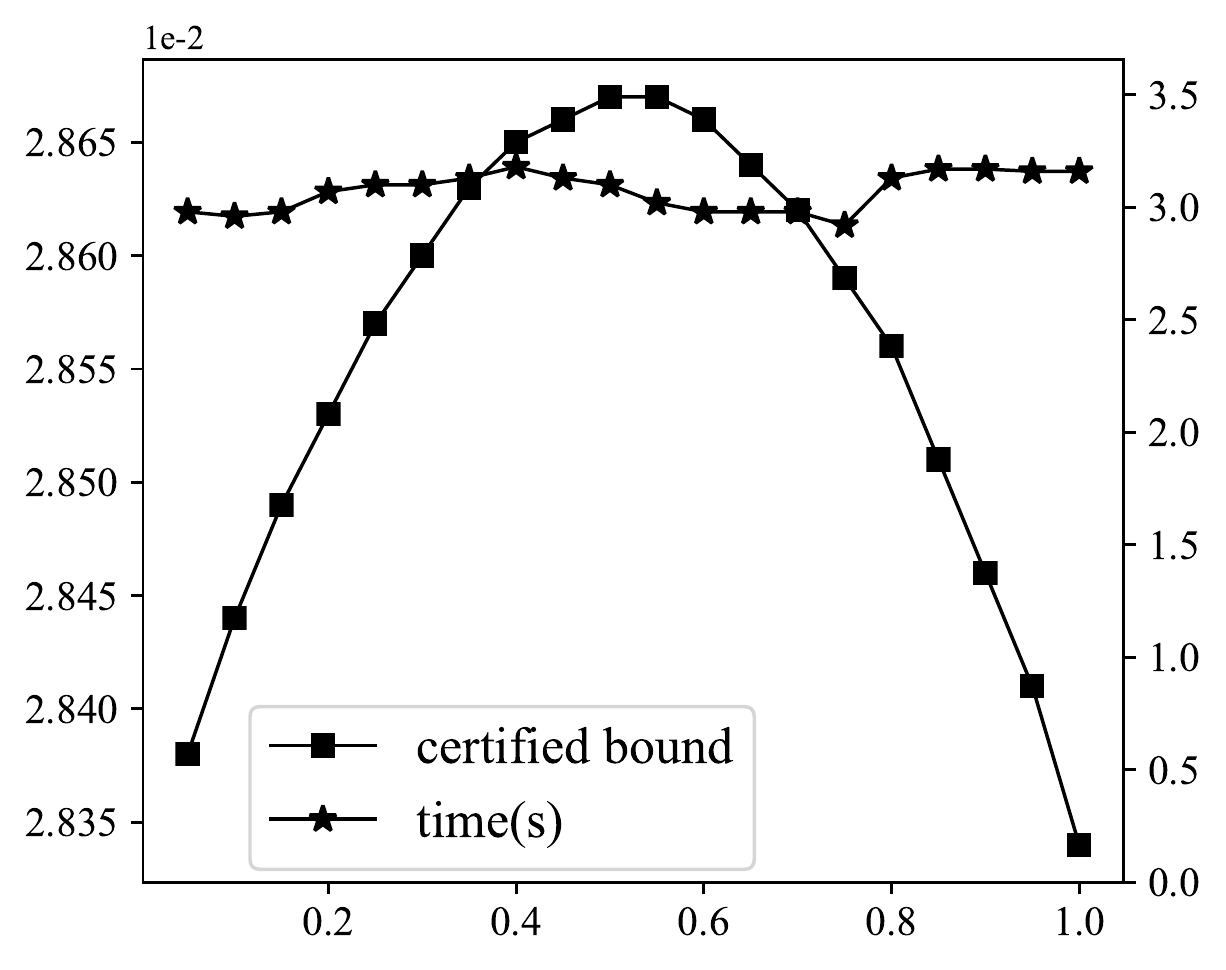}
		\caption{Gradient-based results on $\rm{FNN}_{1\times 200}$ trained on Mnist.}
		\label{fig:GD_mnist_fnn}
	\end{subfigure}
	\hfill
	\begin{subfigure}{0.32\textwidth}
		\includegraphics[width=\textwidth]{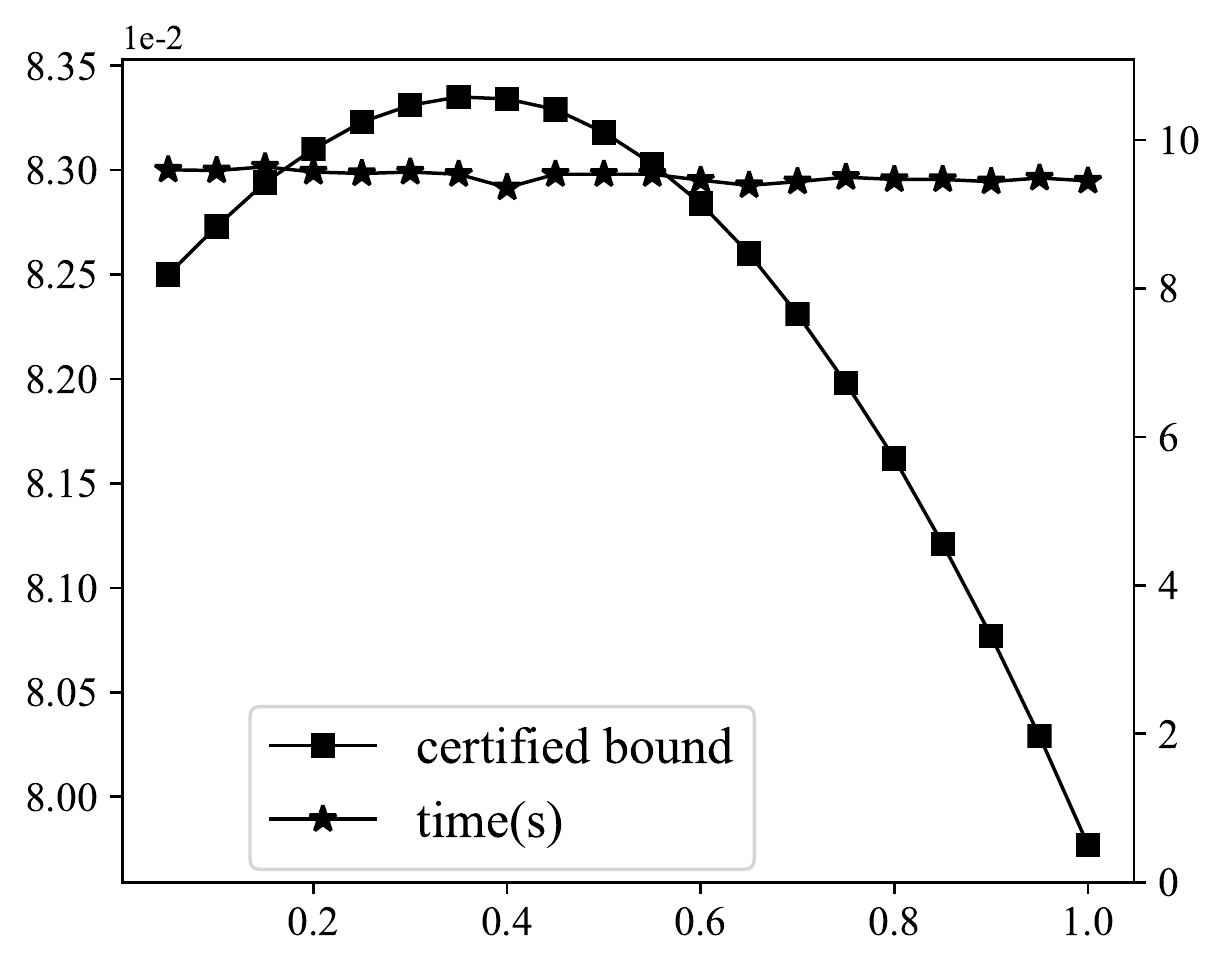}
		\caption{Gradient-based results on $\rm{CNN}_{2-2}$ trained on Fashion Mnist.}
		\label{fig:GD_fashion_mnist_cnn}
	\end{subfigure}
	\hfill
% 	\begin{subfigure}{0.36\textwidth}
% 		\includegraphics[width=\textwidth]{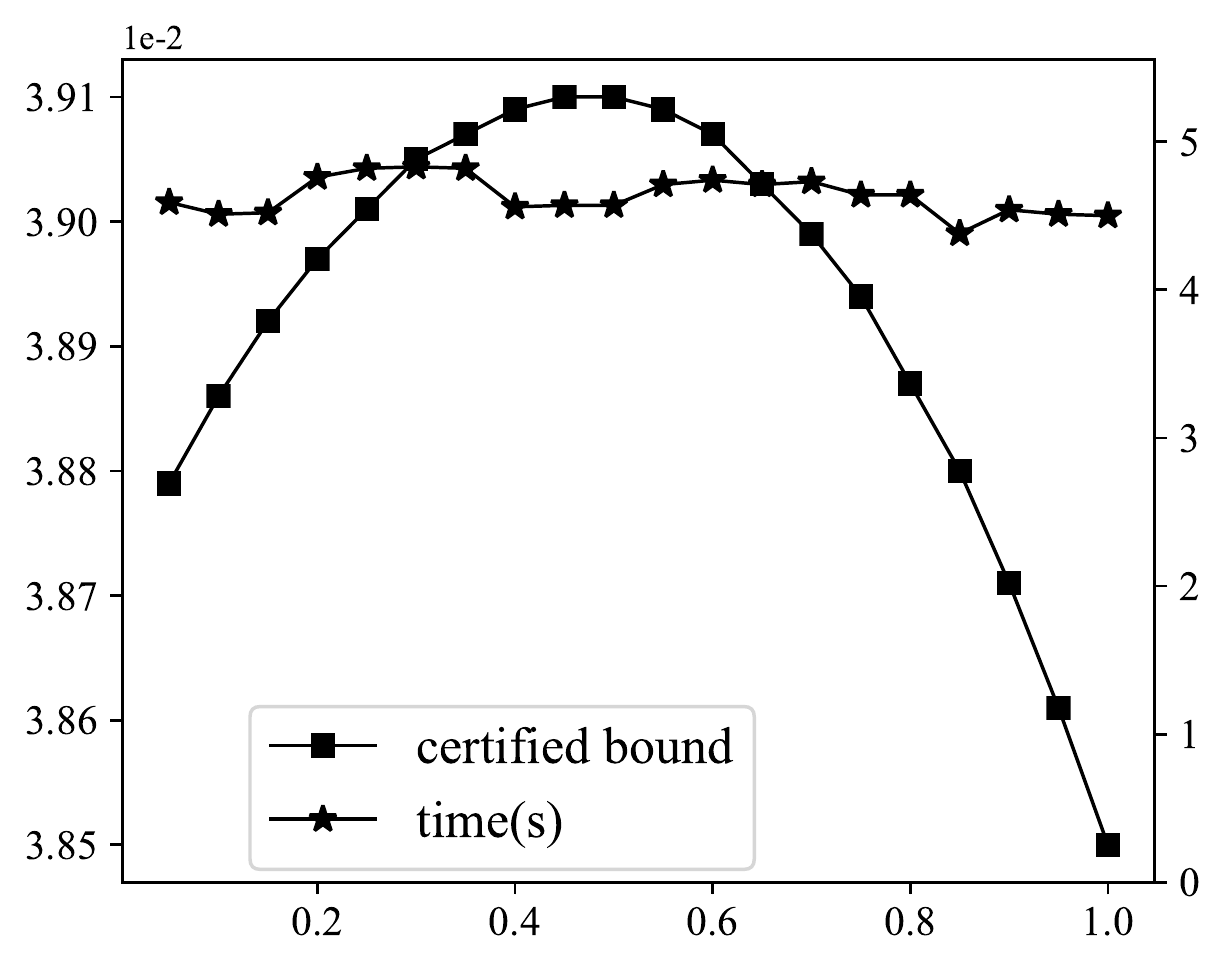}
% 		\caption{Gradient-based results on $\rm{FNN}_{1\times 250}$ trained on Fashion Mnist.}
% 		\label{fig:GD_fashion_mnist_fnn}
% 	\end{subfigure}
% 	\hfill
	\caption{Additional Experimental results: The effect of hyper-parameters in the gradient-based and sampling-based algorithms. The main coordinate denotes certified bounds and the secondary coordinate denotes the time consumed.}
	\label{hyper_para_fig}
	\vspace{-3mm}
\end{figure*}
